# Supplementary material for: Interplay between Federated Learning and Explainable Artificial Intelligence: a Scoping Review
Source: arXiv:2411.05874 source file (2025-04-10)
Supplement: Supplementary file 1 [file supplementary.tex]

\documentclass[conference]{IEEEtran}
\title{Supplementary Material: Appendix for “Interplay between Federated Learning and Explainable Artificial Intelligence: a Scoping Review”}

\author{Luis M. Lopez-Ramos, Florian Leiser, Aditya Rastogi, Steven Hicks, \\ Inga Strümke, Vince I. Madai, Tobias Budig, Ali Sunyaev, and Adam Hilbert\\ On behalf of the VALIDATE consortium}

\usepackage{xr-hyper}
\externaldocument{main} % Replace with your main document’s filename without the .tex extension
\bibliographystyle{IEEEtran} % Or your chosen style

\begin{document}
\maketitle

\appendices

\input{appendices}

\end{document}
